# Supplementary material for: NeRD: Neural 3D Reflection Symmetry Detector
Source: arXiv:2105.03211 source file (2021-04-19)
Supplement: Supplementary file 1 [file table-supplementary-architecture.tex]

\begin{table}[t]
\centering\small

\caption{Summary of the network architecture of SymmetryNet. Unless otherwise specified, batch normalization and ReLU is applied in each convolution layer. The parentheses represent the residue blocks \cite{he2016deep}.}
\label{tab:architecture}
 
\resizebox{.8\linewidth}{!}{%
\begin{tabular}{|c|c|c|}
\hline
\multirow{2}{*}{} & Layer setting                                                                                                            & Output dimension                                                  \\ \cline{2-3} 
                  & input image                                                                                                              & $3 \times H \times W$                                             \\ \hline
\multicolumn{3}{|c|}{\textbf{Backbone Network}}                                                                                                                                                                  \\ \hline
conv0             & $5 \times 5, 32$, 2-stride                                                                                               & $32 \times \frac{H}{2} \times \frac{W}{2}$                        \\ \hline
conv1             & $\begin{pmatrix}3 \times 3, 32\\ 3 \times 3, 32 \end{pmatrix} \times 2$                                                  & $32 \times \frac{H}{2} \times \frac{W}{2}$                        \\ \hline
pooling           & max pooling, 2-stride                                                                                                    & $32 \times \frac{H}{4} \times \frac{W}{4}$                        \\ \hline
conv2             & $\begin{pmatrix}3 \times 3, 32\\ 3 \times 3, 32 \end{pmatrix} \times 3$                                                  & $32 \times \frac{H}{4} \times \frac{W}{4}$                        \\ \hline
conv3             & $3\times3, 32$, no activation                                                                                            & $32 \times \frac{H}{4} \times \frac{W}{4}$                        \\ \hline
\multicolumn{3}{|c|}{\textbf{Feature Warping Module}}                                                                                                                                                            \\ \hline
\multicolumn{2}{|c|}{warp and concatenate}                                                                                                   & $32|\mathcal{M}| \times D \times \frac{H}{4} \times \frac{W}{4}$  \\ \hline
\multicolumn{3}{|c|}{\textbf{Cost Volume Network}}                                                                                                                                                               \\ \hline
3dconv0           & \begin{tabular}[c]{@{}c@{}}$1 \times 1 \times 1, 64$\\ $1 \times 1 \times 1, 64$\\ $3 \times 3 \times 3, 8$\end{tabular} & $8 \times D \times \frac{H}{4} \times \frac{W}{4}$                \\ \hline
3dconv1/0         & $3 \times 3 \times 3, 16$, 2-stride                                                                                      & $8 \times \frac{D}{2} \times \frac{H}{8} \times \frac{W}{8}$      \\ \hline
3dconv1/1         & $3 \times 3 \times 3, 16$                                                                                                & $16 \times \frac{D}{2} \times \frac{H}{8} \times \frac{W}{8}$     \\ \hline
3dconv2/0         & $3 \times 3 \times 3, 32$, 2-stride                                                                                      & $32 \times \frac{D}{4} \times \frac{H}{16} \times \frac{W}{16}$   \\ \hline
3dconv2/1         & $3 \times 3 \times 3, 32$                                                                                                & $32 \times \frac{D}{4} \times \frac{H}{16} \times \frac{W}{16}$   \\ \hline
3dconv3/0         & $3 \times 3 \times 3, 64$, 2-stride                                                                                      & $64 \times \frac{D}{8} \times \frac{H}{32} \times \frac{W}{32}$   \\ \hline
3dconv3/1         & $3 \times 3 \times 3, 64$                                                                                                & $64 \times \frac{D}{8} \times \frac{H}{32} \times \frac{W}{32}$   \\ \hline
3dconv4/0         & $3 \times 3 \times 3, 128$, 2-stride                                                                                     & $128 \times \frac{D}{16} \times \frac{H}{64} \times \frac{W}{64}$ \\ \hline
3dconv4/1         & $3 \times 3 \times 3, 128$                                                                                               & $128 \times \frac{D}{16} \times \frac{H}{32} \times \frac{W}{32}$ \\ \hline
3dconv4/2         & \begin{tabular}[c]{@{}c@{}}deconv $3 \times 3 \times 3, 64$, 2-stride\\ add 3dconv3/1\end{tabular}                       & $64 \times \frac{D}{8} \times \frac{H}{32} \times \frac{W}{32}$   \\ \hline
3dconv3/2         & \begin{tabular}[c]{@{}c@{}}deconv $3 \times 3 \times 3, 32$, 2-stride\\ add 3dconv2/1\end{tabular}                       & $32 \times \frac{D}{4} \times \frac{H}{16} \times \frac{W}{16}$   \\ \hline
3dconv2/2         & \begin{tabular}[c]{@{}c@{}}deconv $3 \times 3 \times 3, 16$, 2-stride\\ add 3dconv1/1\end{tabular}                       & $16 \times \frac{D}{2} \times \frac{H}{8} \times \frac{W}{8}$     \\ \hline
3dconv1/2         & \begin{tabular}[c]{@{}c@{}}deconv $3 \times 3 \times 3, 8$, 2-stride\\ add 3dconv0/1\end{tabular}                        & $8 \times D \times \frac{H}{4} \times \frac{W}{4}$                \\ \hline
3dconv5           & $3\times3\times3, 1$, softmax                                                                                            & $1 \times D \times \frac{H}{4} \times \frac{W}{4}$                \\ \hline
\multicolumn{3}{|c|}{\textbf{Depth Map Regression}}                                                                                                                                                              \\ \hline
\multicolumn{2}{|c|}{Expectation (soft argmin)}                                                                                              & $\frac{H}{4} \times \frac{W}{4}$                                  \\ \hline
\multicolumn{2}{|c|}{Bilinear Upsample}                                                                                                      & $H \times W$                                                      \\ \hline
\multicolumn{2}{|c|}{$\ell_1$ Regression}                                                                                                    & N/A                                                               \\ \hline
\end{tabular}%
}
\end{table}
