# Supplementary material for: NeRD: Neural 3D Reflection Symmetry Detector
Source: arXiv:2105.03211 source file (2021-04-19)
Supplement: Supplementary file 2 [file table-supplementary-multiaxis.tex]

\begin{table*}[tpb]
\centering

\setlength{\tabcolsep}{1.2mm}

\resizebox{\textwidth}{!}{%
\begin{tabular}{l|cccc|cccc|cccc}
\hline
\multirow{2}{*}{}   & \multicolumn{4}{c|}{Mean $\ell_1$}                                                                                            & \multicolumn{4}{c|}{Median $\ell_1$}                                                                                          & \multicolumn{4}{c}{RMSE}                                                                                                      \\ \cline{2-13} 
                    & \scriptsize $|\mathcal{M}|=1$ & \scriptsize $|\mathcal{M}|=2$ & \scriptsize $|\mathcal{M}|=3$ & \scriptsize $|\mathcal{M}|=4$ & \scriptsize $|\mathcal{M}|=1$ & \scriptsize $|\mathcal{M}|=2$ & \scriptsize $|\mathcal{M}|=3$ & \scriptsize $|\mathcal{M}|=4$ & \scriptsize $|\mathcal{M}|=1$ & \scriptsize $|\mathcal{M}|=2$ & \scriptsize $|\mathcal{M}|=3$ & \scriptsize $|\mathcal{M}|=4$ \\ \hline
Plane               & 0.0278                        & 0.0146                        & 0.0154                        & \textbf{0.0082}               & 0.0190                        & 0.0075                        & 0.0080                        & \textbf{0.0039}               & 0.0407                        & 0.0256                        & 0.0264                        & \textbf{0.0153}               \\
Bench               & 0.0211                        & \textbf{0.0104}               & 0.0139                        & 0.0109                        & 0.0120                        & \textbf{0.0037}               & 0.0065                        & 0.0054                        & 0.0355                        & 0.0240                        & 0.0272                        & \textbf{0.0215}               \\
Cabinet$^\sharp$    & 0.0252                        & 0.0111                        & 0.0111                        & \textbf{0.0087}               & 0.0145                        & 0.0059                        & 0.0055                        & \textbf{0.0030}               & 0.0415                        & \textbf{0.0206}               & 0.0219                        & 0.0211                        \\
Car                 & 0.0196                        & 0.0113                        & \textbf{0.0094}               & 0.0136                        & 0.0125                        & 0.0056                        & \textbf{0.0032}               & 0.0063                        & 0.0311                        & \textbf{0.0220}               & 0.0224                        & 0.0265                        \\
Chair               & 0.0215                        & \textbf{0.0101}               & 0.0111                        & 0.0176                        & 0.0121                        & \textbf{0.0050}               & 0.0059                        & 0.0077                        & 0.0368                        & \textbf{0.0191}               & 0.0202                        & 0.0316                        \\
Monitor$^\sharp$    & 0.0323                        & 0.0125                        & \textbf{0.0084}               & 0.0123                        & 0.0214                        & 0.0063                        & \textbf{0.0040}               & 0.0065                        & 0.0474                        & 0.0239                        & \textbf{0.0152}               & 0.0233                        \\
Lamp                & 0.0167                        & \textbf{0.0085}               & 0.0139                        & 0.0137                        & 0.0109                        & \textbf{0.0043}               & 0.0073                        & 0.0073                        & 0.0261                        & \textbf{0.0171}               & 0.0240                        & 0.0235                        \\
Speaker$^\sharp$    & 0.0304                        & 0.
0153                        & \textbf{0.0085}               & 0.0139                        & 0.0210                        & 0.0073                        & \textbf{0.0045}               & 0.0065                        & 0.0441                        & 0.0279                        & \textbf{0.0168}               & 0.0252                        \\
Firearm             & 0.0289                        & \textbf{0.0140}               & 0.0186                        & 0.0154                        & 0.0184                        & \textbf{0.0064}               & 0.0081                        & 0.0080                        & 0.0447                        & 0.0272                        & 0.0336                        & \textbf{0.0264}               \\
Couch               & 0.0251                        & \textbf{0.0086}               & 0.0145                        & 0.0111                        & 0.0163                        & \textbf{0.0040}               & 0.0069                        & 0.0059                        & 0.0372                        & \textbf{0.0157}               & 0.0267                        & 0.0199                        \\
Table$^\sharp$      & 0.0255                        & 0.0148                        & 0.0127                        & \textbf{0.0079}               & 0.0150                        & 0.0071                        & 0.0067                        & \textbf{0.0040}               & 0.0399                        & 0.0263                        & 0.0241                        & \textbf{0.0163}               \\
Phone$^\sharp$      & 0.0333                        & 0.0158                        & \textbf{0.0104}               & 0.0137                        & 0.0237                        & 0.0079                        & \textbf{0.0051}               & 0.0063                        & 0.0463                        & 0.0279                        & \textbf{0.0196}               & 0.0252                        \\
Watercraft$^\sharp$ & 0.0361                        & 0.0190                        & 0.0144                        & \textbf{0.0097}               & 0.0216                        & 0.0084                        & 0.0069                        & \textbf{0.0049}               & 0.0547                        & 0.0337                        & 0.0258                        & \textbf{0.0184}               \\ \hline
Average             & 0.0263                        & 0.0127                        & 0.0125                        & \textbf{0.0120}               & 0.0162                        & 0.0059                        & 0.0059                        & \textbf{0.0055}               & 0.0410                        & 0.0242                        & 0.0236                        & \textbf{0.0229}               \\ \hline
\end{tabular}%
}
\caption{Performance of SymmetryNet with multiple symmetry transformations. Let $\mathcal{M}$ be the set of symmetry transformations that the objects admit, including the identity $\M_1=\I$. When $|\mathcal{M}|=1$, we concatenate the image feature with the one-hot features on the depth dimension to construct the cost volume, while for $|\mathcal{M}|=2$, $|\mathcal{M}|=3$, $|\mathcal{M}|=4$, we gradually add the warped features to the cost volume from the transformations $\M_2=\mathrm{diag}(-1, 1, 1)$, $\M_3=\mathrm{diag}(1, -1, 1)$, and $\M_4=\mathrm{diag}(-1, -1, 1)$.  We label the categories with $\sharp$ if both of the mean $\ell_1$ errors in the columns of $|\mathcal{M}|=3$ and $|\mathcal{M}|=4$ are smaller than the error in the column of $|\mathcal{M}|=2$, indicating many objects in these categories admit additional symmetry.  The lowest error in each comparison is highlighted in \textbf{boldface}.}
\label{tab:multiaxis}

\vspace{5mm}

\end{table*}
